# Supplementary material for: Improving Knowledge Distillation via Regularizing Feature Norm and Direction
Source: arXiv:2305.17007 source file (2023-05-26)
Supplement: Supplementary file 1 [file suppl_ablation.tex]

\begin{table}
    \begin{subtable}[h]{0.28\textwidth}
        
        \small
        \centering
        \begin{tabular}{lc}
        case &  acc.\\
        \hline
        \toprule
        \textit{baseline} & 67.65\\
        MSE & 69.05\\
        SIFN & 69.32\\
        &\\
        &\\
        \end{tabular}
        \vspace{1.5mm}
        \caption{Regularizing feature \textbf{norm} only improve accuracy.}\label{norm}
    \end{subtable}
    \hfill
    \begin{subtable}[h]{0.38\textwidth}
        \setlength\tabcolsep{1.5pt}
        
        \small
        \centering
        \begin{tabular}{lcc}
        case & R50$\rightarrow$MV2 & R56$\rightarrow $R20\\
        \hline
        \toprule
        \textit{baseline} & 67.65 & 70.66\\
        % \hline
        % \textit{only direction} & ~ & ~\\
        cosine & 69.18 & 71.75\\
        InfoNCE   & 69.06 & 70.73\\
        &\\
        &\\
        \end{tabular}
        \vspace{1.5mm}
        \caption{Regularizing feature \textbf{direction} only. \textit{Cosine} is suitable for more diverse nets.}\label{direction}
    \end{subtable}
    \hfill
    \begin{subtable}[h]{0.30\textwidth}
        \setlength\tabcolsep{1.5pt}
        
        \small
        \centering
        \begin{tabular}{lc}
        case &  acc.\\
        \hline
        \toprule
        cosine w/ MSE & 68.62\\
        cosine w/ SIFN & 69.07\\
        InfoNCE w/ MSE & 68.47\\
        InfoNCE w/ SIFN & 68.71\\
        ND           & \colorbox{lightgray}{\textbf{70.10}}\\
        \end{tabular}
        \vspace{1.5mm}
        \caption{Regularizing \textbf{direction w/ norm}. ND works the best.}\label{dir-norm}
    \end{subtable}
    \hfill
    \begin{subtable}[h]{0.35\textwidth}
        
        \small
        \centering
        \begin{tabular}{ccc}
        \textit{k} & R50$\rightarrow$MV2 & R56$\rightarrow $R20\\
        \hline
        \toprule
        -0.5 & 69.46 & 71.57\\
        0.0    & \colorbox{lightgray}{\textbf{70.10}} & \colorbox{lightgray}{\textbf{72.53}}\\
        0.5	 & 70.23	& 71.86\\
        1.0	 & 69.72	& 71.79\\
        1.5	 & 68.49	& 71.74\\
        \end{tabular}
        \vspace{1.5mm}
        \caption{\textbf{scale teacher norm}. use the teacher norm as the learning objective.}
        \label{tea-norm}
    \end{subtable}
    \hfill
    \begin{subtable}[h]{0.25\textwidth}
        
        \small
        \centering
        \begin{tabular}{lc}
        case &  acc.\\
        \hline
        \toprule
        % \textit{only norm} & ~\\
        easy samples & 72.01\\
        all samples  & \colorbox{lightgray}{\textbf{71.98}}\\
         &\\
         &\\
         &\\
        \end{tabular}
        \vspace{1.5mm}
        \caption{\textbf{sample strategy} has little effect on distillation.}\label{sample}
    \end{subtable}
    \hfill
    \begin{subtable}[h]{0.18\textwidth}
        
        \small
        \centering
        \begin{tabular}{cc}
        $\beta$ &  acc.\\
        \hline
        \toprule
        0.5  & 69.37\\
        1.0  & 68.64\\
        2.0  & 69.19\\
        3.0  & 67.32\\
        4.0  & 68.58\\
        \end{tabular}
        \vspace{1.5mm}
        \caption{Sensitivity of \textbf{$\beta$}. $(\alpha=1.0)$.}\label{beta}
    \end{subtable}
    \hfill
    \begin{subtable}[h]{0.18\textwidth}
        
        \small
        \centering
        \begin{tabular}{cc}
        $\alpha$ &  acc.\\
        \hline
        \toprule
        0.5  & 68.61\\
        1.0  & 68.69\\
        2.0  & 69.07\\
        3.0  & \colorbox{lightgray}{\textbf{70.10}}\\
        4.0  & 69.83\\
        \end{tabular}
        \vspace{1.5mm}
        \caption{ Sensitivity of \textbf{$\alpha$}. $(\beta=0.5)$.}\label{alpha}
    \end{subtable}
\vspace{2.5mm}
\caption{\textbf{Ablation experiments on CIFAR-100.} We report accuracy on the test set. If not specified, the default is: the teacher and student are ResNet-50 and MobileNet-V2, respectively, and student trained by Eq.8. We count the mean of the teacher's embedding features for each category on the whole training set as the category center. Default settings are marked in \colorbox{lightgray}{gray}.}
\label{tab:suppl_ablation}
\end{table}
