# Supplementary material for: Improving Knowledge Distillation via Regularizing Feature Norm and Direction
Source: arXiv:2305.17007 source file (2023-05-26)
Supplement: Supplementary file 2 [file appendix.tex]

\section{Appendix}
\subsection{A. Implementation Details}
\textbf{CIFAR-100.} Our implementation follows the practice in ~\cite{tian2019contrastive}: 4 pixels are padded on each side, and a $32\times32$ crop is randomly sampled from the padded images or its horizontal flip. We initialize the weights as in and train all students from scratch, and teachers loads the available public weights. The students are trained with a mini-batch size of 128 on two GPUs for 240 epochs with SGD. The weight decay and the momentum are set to 5e-4 and 0.9. We start with a learning rate of 0.1 for ResNet and WRN, 0.02 for MobileNet-V2 and ShuffleNet, and divide it by 10 at 150, 180, and 210 epochs. The temperature is set as 4 and the weight for the cross-entropy loss is set to 1.0, $\alpha$ and $\beta$ in Eq.~\ref{eq5} are manually tuned. And we use a 20 epochs linear warmup for $\mathcal{L}_{KD}$ in all experiments.

\textbf{ImageNet.} We constructed two training strategies on the dataset. For base version, our implementation follows the standard practice. We use SGD with a mini-batch size of 256. The learning rate start from 0.1 and is divided every 30 epochs, and the students are trained for up to 100 epochs. We use a weight decay of 1e-4 and a momentum of 0.9. Teachers loads \textbf{PyTorch} pre-trained weight. The temperature is set as 1 and the weight for the cross-entropy loss is set to 1.0. For stronger training strategy are summary in Table~\ref{tab:strategy}.
\input{tables/train-strategy}
