# Supplementary material for: Improving Knowledge Distillation via Regularizing Feature Norm and Direction
Source: arXiv:2305.17007 source file (2023-05-26)
Supplement: Supplementary file 3 [file suppl_dir_norm.tex]

% \begin{table}[h]
%     \centering
%     \caption{
%     }
%     \vspace{1mm}
%         \renewcommand{\arraystretch}{1.2}
%         % \setlength\tabcolsep{1.5pt}
%         \resizebox{0.9\textwidth}{!}{%
%         % \small
%         \begin{tabular}{c|c|cc|cc|ccccc}
%         \hline
%         methods & KD & \multicolumn{2}{c}{only Norm} & \multicolumn{2}{|c}{only Direction} & \multicolumn{5}{|c}{Direction w/ Norm}\\
%         \cline{2-11}
%         \hline
%         \textit{baseline} & $\checkmark$ & ~ & ~ & ~ & ~\\
%         \hline
%         MSE               & ~ & $\checkmark$ & ~ & ~ & ~ & $\checkmark$ & ~ & $\checkmark$\\
%         SIFN              & ~ & ~ & $\checkmark$ & ~ & ~ & ~ & $\checkmark$ & ~ & $\checkmark$\\
%         \hline
%         cosine            & ~ & ~ & ~ & $\checkmark$ & ~ & $\checkmark$ & $\checkmark$\\
%         InfoNCE           & ~ & ~ & ~ & ~ & $\checkmark$ & ~ & ~ & $\checkmark$ & $\checkmark$\\
%         \hline
%         \textbf{ND}                & ~ & ~ & ~ & ~ & ~ & ~ & ~ & ~ & ~ & $\checkmark$\\
%         \hline
%         Acc (\%) & 67.65 & 69.05 & 69.32 & 69.18 & 69.06 & 68.62 & 69.07 & 68.47 & 68.71 & \textbf{70.10}\\
%         \hline
%         \end{tabular}
%     }
%        %\vspace{1.5mm}
%         \label{tab:suppl_dir_norm}
% \end{table}

\begin{table}[h]
\centering
    \caption{}
    \vspace{1mm}

        \resizebox{0.7\textwidth}{!}{%
        % \small
        \begin{tabular}{ccccccc}
        \hline
        \textit{baseline} & \multicolumn{2}{c}{Regular Norm} & \multicolumn{2}{c}{Regular Direction} & ours & ~\\
        KD & MSE & SIFN & cosine & InfoNCE & \textbf{ND} & Acc (\%)\\
        \hline
        $\checkmark$ & ~ & ~ & ~ & ~ & ~ & 67.65\\
        ~ & $\checkmark$ & ~ & ~ & ~ & ~ & 69.05\\
        ~ & ~ & $\checkmark$ & ~ & ~ & ~ & 69.32\\
        ~ & ~ & ~ & $\checkmark$ & ~ & ~ & 69.18\\
        ~ & ~ & ~ & ~ & $\checkmark$ & ~ & 69.06\\
        ~ & $\checkmark$ & ~ & $\checkmark$ & ~ & ~ & 69.06\\
        ~ & ~ & $\checkmark$ & $\checkmark$ & ~ & ~ & 69.06\\
        ~ & $\checkmark$ & ~ & ~ & $\checkmark$ & ~ & 69.06\\
        ~ & ~ & $\checkmark$ & ~ & $\checkmark$ & ~ & 69.06\\
        ~ & ~ & ~ & ~ & ~ & $\checkmark$ & \textbf{70.10}\\
        \hline
        \end{tabular}
    }
    \label{tab:suppl_dir_norm}
\end{table}
